# Supplementary material for: NADI 2022: The Third Nuanced Arabic Dialect Identification Shared Task
Source: arXiv:2210.09582 source file (2022-10-20)
Supplement: Supplementary file 1 [file appendix.tex]

\newpage
\appendixpage
% \addappheadtotoc
\numberwithin{figure}{section}
\numberwithin{table}{section}

\section{Shared Task Datasets}\label{appx:data_eval}

\input{tables/subtask_1_distribution}
